# Supplementary material for: Numerical Discretization Methods for the Discounted Linear Quadratic Control Problem
Source: arXiv:2407.18769 source file (2024-07-26)
Supplement: Supplementary file 1 [file AppendixProofs.tex]

%% %%%%%%%%%%%%%%%%%%%%%%%%%%%%%%%%%%%%%%
\section{Proofs}
